# Supplementary material for: Visually Guided Sound Source Separation and Localization using Self-Supervised Motion Representations
Source: arXiv:2104.08506 source file (2021-04-17)
Supplement: Supplementary file 1 [file supp_sep_2diff_AVE.pdf]

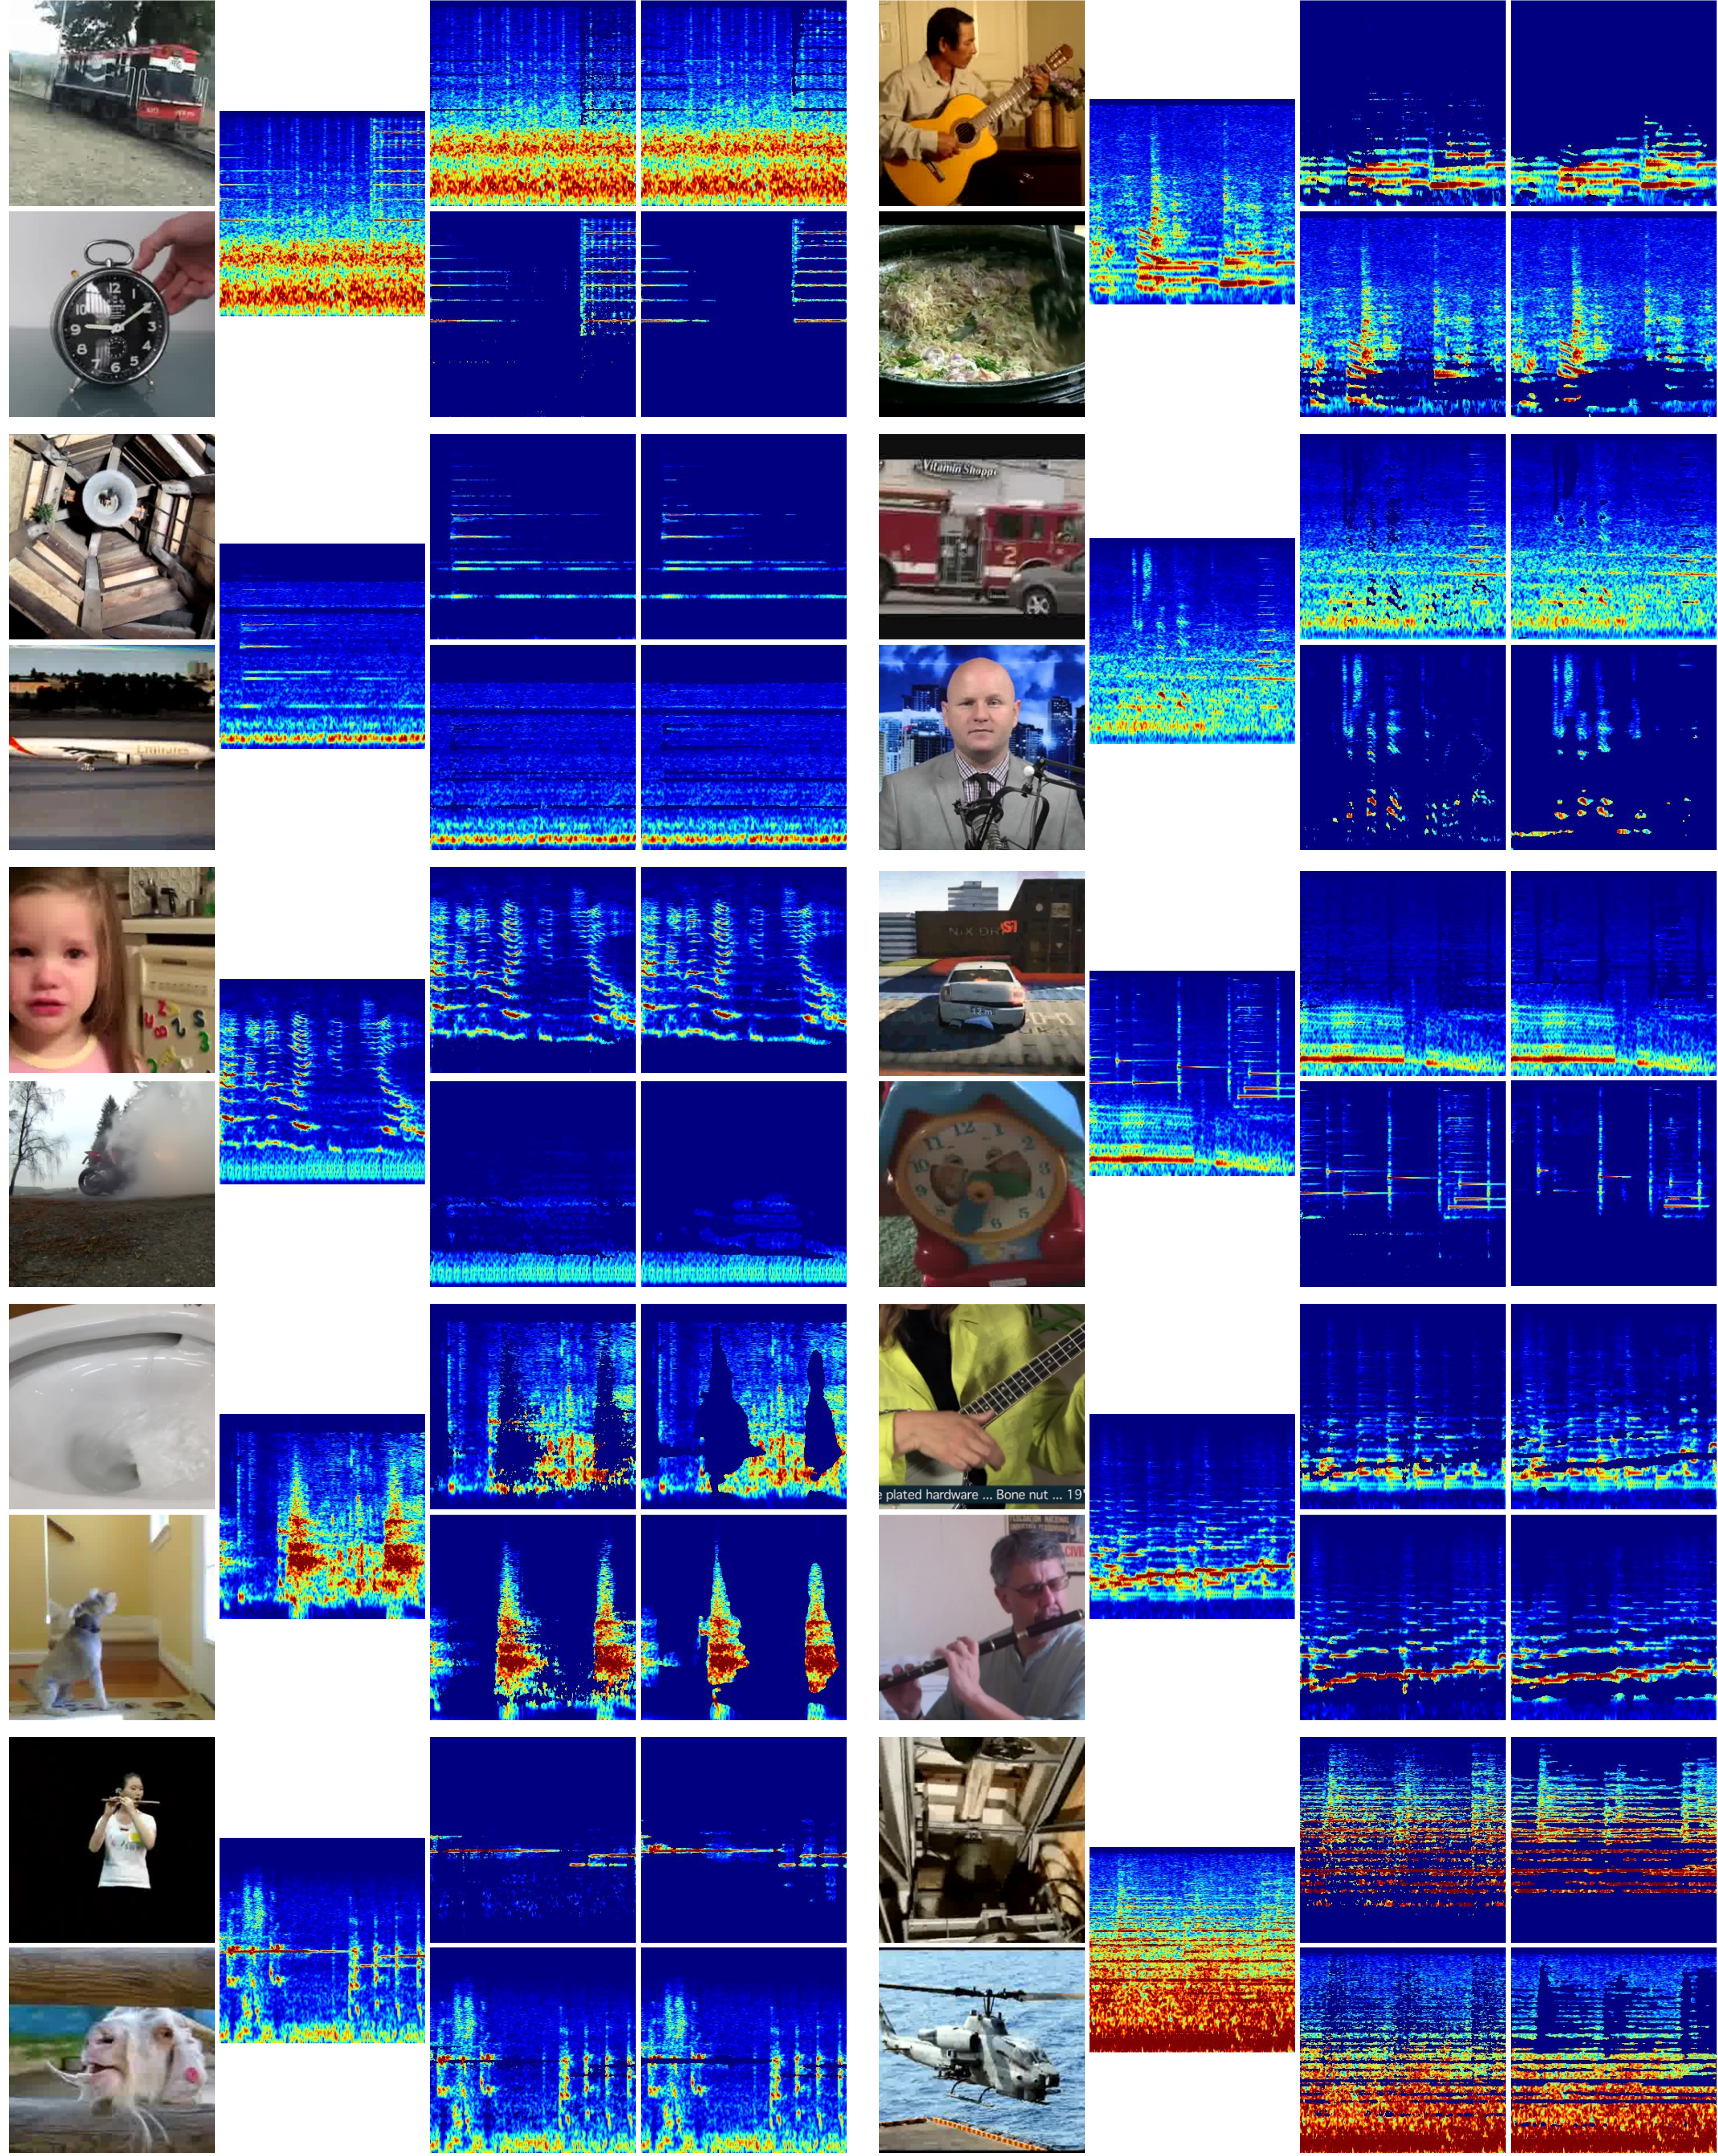

Video frames

$X_{mix}$

Ground truth

AMnet

Video frames

$X_{mix}$

Ground truth

AMnet
